# Supplementary material for: xLAM: A Family of Large Action Models to Empower AI Agent Systems
Source: arXiv:2409.03215 source file (2024-09-05)
Supplement: Supplementary file 1 [file appendix.tex]

\section{Model Training Details} \label{appendix:training}

Our training code leverages the public HuggingFace Transformers libaray~\citep{wolf2020transformers}, where we adopt the distributed supervised fine-tuning approach and capitalize on the capabilities of our data collection pipeline.  We diversify the random seeds based on the process ID when data parallelism is utilized across multiple devices. This careful management of the seeding process helps maintain a balanced distribution of data by partitioning, shuffling and interleaving data across devices while preserving randomness, thus enhancing the robustness and reproducibility of our training procedure. 

The fine-tuning of general xLAM models is executed on H100 pods, each equipped with eight Nvidia H100 GPUs, using a fully-finetuning framework that implements the fully sharded data parallel algorithm \citep{zhao2023pytorch}. We set a batch size of four per GPU and a gradient accumulation step of three. The training uses a learning rate ranging from $2 \times 10^{-6}$, to $2 \times 10^{-4}$, and a maximum sequence length of 8192. For xLAM-8x22b-r, we incorporate LORA~\citep{hu2021lora,dettmers2023qlora} to better preserve the model's original capacities and mitigate catastrophic forgetting.
Additionally, we utilize a cosine learning rate scheduler with 100 warm-up steps to optimize performance.

The xLAM-FC models focus on various categories of function-calling agents, including simple, multiple, parallel, and parallel multiple. These categories are designed to challenge and enhance the models' capabilities in different usage scenarios. For example, a simple query like retrieving the weather for a single location, such as ``What is the weather in Palo Alto today?'' which can be answered by calling \texttt{get\_weather("Palo Alto", "today")}. Multiple queries involve selecting the most appropriate function from several provided APIs, while parallel queries require executing multiple function calls simultaneously in response to a single user query. %
Additionally, the models are trained on relevance detection, which assesses the alignment between function calls, execution results, and query objectives.

The xLAM-FC models are trained using the following hyperparameters: a learning rate of $5 \times 10^{-6}$, two epochs, and the AdamW optimizer. Other settings include a per-device batch size of six, two gradient accumulation steps, a cosine learning rate scheduler with 50 warmup steps, and the bfloat16 (BF16) data type.
